# Supplementary material for: Single Round-trip Hierarchical ORAM via Succinct Indices
Source: arXiv:2208.07489 source file (2024-06-13)
Supplement: Supplementary file 1 [file additional_proofs.tex]

\section{Additional Proofs}

\subsection{Proof for Lemma \ref{lem:shortqueue}}
\label{app:lemma8}
We break down Lemma \ref{lem:shortqueue} into its components of fail rate, performance and security.
The algorithm fails if the temporary client storage exceeds $c\cdot \sqrt{n}$ for some constant $c$.
\begin{lemma}
On input array length $n$, \shortqueue fails with probability negligible in $n$.
\label{lem:fail_rate}
\end{lemma}
Before proving the result we require some probability tools.
\begin{definition}[Negative Association]
The random variables $X_1, \ldots, X_n$ are negatively associated if for all disjoint sets $ \mathbf{X}_1, \mathbf{X}_2 \subseteq \{X_1, \ldots, X_n\}$,
\begin{align*}
    \mathrm{E}[f(\mathbf{X}_1) \cdot g(\mathbf{X}_2)] \leq \mathrm{E}[f(\mathbf{X}_1)] \cdot \mathrm{E}[g(\mathbf{X}_2)],
\end{align*}
for all functions $f$ and $g$ that both non-increasing or both non-decreasing.
\end{definition}
This property, along with the following result, will be used to bound the size of the queues. 
\begin{lemma}[Lemma 2 of \cite{dubhashi1996balls}]
Let $X_1, \ldots, X_n$ be negatively associated random variables.
Then for non-decreasing functions $f_1, \ldots, f_k$ over disjoint sets $S_1, \ldots, S_k \subseteq \{ X_1, \ldots, X_n$\},
\begin{align*}
    \mathrm{E}\left[\prod_{i\in[k]} f_i(S_i) \right] &\leq \prod_{i\in[k]} \mathrm{E}\left[ f_i(S_i) \right]
\end{align*}
\label{lem:neg_ass_bounds}
\end{lemma}
Finally, we need the following result from Queuing Theory.
\begin{theorem}
Let $Q$ be a queue with batched arrival rate $1-\varepsilon$ and departure rate 1 and let $q_t$ be the size of the queue after $t$ batches of arrival. 
Then, for all $\varepsilon > 0, \mathrm{E}[e^{q_t}] \leq 2$.
\label{thm:queue_bound}
\end{theorem}

\begin{proof}[proof of Lemma \ref{lem:fail_rate}]
The goal is to bound the combined size of the queues during the execution of the algorithm.
To accomplish this, we construct a variant of \shortqueue that has the same functionality and fail rate.
We will prove that the fail rate for this variant is negligible.
The variant splits the input buckets $I_1, \ldots, I_{\sqrt{n}}$ in half and executes the first step of \shortqueue by reading the half-buckets in $2\sqrt{n}$ rounds.
After a half-bucket has been downloaded, \textit{one} item from each queue is uploaded to the temporary bucket at the server.
This is the only difference between the two.
As the ratio between the arrival and eviction rates at each queue is the same for both algorithms, they have identical fail rates. 
The variation allows us to use Theorem \ref{thm:queue_bound} with $\varepsilon = 0.5$.

Fixing notation, let $I^{\prime}_{2i}$ denote the first half of $I_{i}$, $I^{\prime}_{2{i+1}}$ denote the second half of $I_{i}$ and $X_{i,j}$ denote the number of addresses from $I^{\prime}_i$ that are placed in $Q_j$.
As the addresses from the input buckets are uniformly distributed across $Q_1,\ldots, Q_{\sqrt{n}}$, with $|I^{\prime}_i| = \sqrt{n}/2$, it holds that 
\begin{align}
    \mathrm{E}[X_{i,j}] = \frac{1}{2}.
    \label{eqn:arrival_rate}
\end{align}
Now, let $Y_{i,j}$ denote the length of $Q_j$ after $I^{\prime}_i$ has been read from the server.
Note that $Y_{i,j}$ is a non-decreasing function of the set of variables $\{X_{1,j}, \ldots, X_{i,j}\}$.
Let $Y_i = \sum_{j=1}^{\sqrt{n}} Y_{i,j}$.
To complete the proof, we need to bound ${Y_i}$ for all $2\sqrt{n}$ rounds.

The random variables $X_{i,1}, \ldots, X_{i,q}$ follow a balls-in-bins process.
Therefore, by Theorem 3.2 of \cite{dubhashi1996balls}, the variables are negatively associated.
Further, for all $i \neq j$, the sets $\{X_{i,1}, \ldots, X_{i,q}\}$ and $\{X_{j,1}, \ldots, X_{j,q}\}$ are mutually independent.
Therefore, the $Y_{i,j}$ are non-decreasing functions of disjoint sets of negatively associated random variables.
By Markov's Inequality,
\begin{align}
    \Pr[Y_i > c\cdot \sqrt{n}]
        &= \Pr[e^{\varepsilon Y_i}  > e^{\varepsilon c\cdot \sqrt{n}}] \nonumber\\
        &\leq e^{-\varepsilon c\cdot \sqrt{n}} \mathrm{E}\left[e^{\varepsilon Y_i}\right].
        \label{eqn:markov_bound}
\end{align}
By Equation \ref{eqn:arrival_rate}, the batched arrival rate is 0.5 and the departure rate is 1.
Therefore, by Theorem \ref{thm:queue_bound}, with $\varepsilon = 0.5$, 
\begin{align*}
    \mathrm{E}\left[e^{0.5 \cdot Y_i}\right] &= \mathrm{E}\left[\prod_{i=j}^{\sqrt{n}}e^{0.5 \cdot Y_{i,j}}\right] \\
    &\leq \prod_{j=1}^{\sqrt{n}} \mathrm{E}\left[ e^{0.5 \cdot Y_{i,j}} \right] \\ 
    &\leq 2^{\sqrt{n}}.
\end{align*}
The second inequality follows from Lemma \ref{lem:neg_ass_bounds}.
Thus, by inequality \ref{eqn:markov_bound}, with $\varepsilon=0.5$, 
\begin{align*}
    \Pr[Y_i > c\cdot \sqrt{n}] &\leq e^{-(c\cdot e/(1+e)-\ln 2)\sqrt{n}}.
\end{align*}
Therefore, by setting $c>(1+1/\varepsilon)\ln 2e$, $Y_i=\mathcal{O}(\sqrt{n})$ with probability at most $e^{-\mathcal{O}(1)\sqrt{n}}$.
Taking a union bound across all $2\sqrt{n}$ timesteps completes the result.
\end{proof}

We cover bandwidth and memory with the following result.
\begin{lemma}
On an input array of length $n$, the \shortqueue completes in $7n$ blocks of bandwidth and, on the condition that it does not fail, requires $\mathcal{O}(B \cdot \sqrt{n})$ bits of temporary private memory.
\end{lemma}
\begin{proof}
The memory claim comes from Lemma \ref{lem:fail_rate} and our definition of failure.
For the bandwidth, the first component of the algorithm downloads $n$ address and uploads $2n$ addresses.
The second component, in a sequence of rounds, downloads the full temporary array of length $2n$ and uploads it to the output array.
This leads to a total bandwidth cost of $7n$.
\end{proof}

\begin{lemma}
The \shortqueue is oblivious on functionality dummy shuffle (\textup{Definition} \ref{def:dummy_shuffle}).
\end{lemma}
\begin{proof}
We need to demonstrate that the access patterns produced by \shortqueue on two distinct inputs $\pi_1$ and $\pi_2$ are computationally indistinguishable to the adversary.
Let $\{I^{b}_i\}_{i \in \sqrt{n}}$ denote the input buckets for the execution of \shortqueue on $\pi_b$ for $b\in\{1,2\}$.
Both sets of input buckets are independent of their corresponding input permutations.
Similarly, let $X^{b}_{i,j}$ denote the number of addresses from $I^{b}_i$ that are placed in $Q^{b}_j$ for $b \in \{1,2\}$.
As the addresses are assigned uniformly at random to the sets $\{I^{b}_i\}_{i \in \sqrt{n}}$, $X^{1}_{i,j}$ is independent of $X^{2}_{i,j}$.
Therefore, for a fixed input array, the fail rate, which is observable to the adversary, is independent of the input permutation.

The set of buckets $\{I^{b}_i\}_{i \in \sqrt{n}}$ is independent of the input permutation.
Thus, the initial phase of downloading the input array appears as a sequence of uniformly random accesses.
The remaining accesses in the algorithm are identical for all inputs of the same length.
This completes the proof.
\end{proof}
